# Supplementary material for: LEGO: Synergizing Expert GraphRAG and Expert Chain-of-Thought for Legal Reasoning
Source: arXiv:2609.27009 source file (2026-10-04)
Supplement: Supplementary file 2 [file appendix_pfc_case_study_detailed.tex]

% This root-level file is deprecated/placeholder.
% The actual appendix content lives in: latex/appendix_pfc_case_study_detailed.tex
% Kept as a stub to avoid accidental inclusion of outdated duplicates.
