# Supplementary material for: LEGO: Synergizing Expert GraphRAG and Expert Chain-of-Thought for Legal Reasoning
Source: arXiv:2609.27009 source file (2026-10-04)
Supplement: Supplementary file 4 [file appendix_synergy.tex]

% Appendix-only: detailed synergy analysis between retrieval and reasoning.

\section*{Appendix: Additional Synergy Analysis}
\phantomsection
\label{sec:appendix_synergy}

This appendix provides the detailed analysis behind our synergy claims between retrieval and reasoning.

\paragraph{Quantifying synergy between retrieval and reasoning.}
We formalise two synergy quantities used throughout the paper. Let $M_0$ denote the baseline system (no retrieval, no expert reasoning), let $M_R$ denote the retrieval-only variant (ExpertGraphRAG with free-form CoT), let $M_C$ denote the reasoning-only variant (a strong retriever with our single-pass ExpertCoT), and let $M_{R+C}$ denote the full system that combines both. For any evaluation metric $s(\cdot)$ (here, Acc and F1 on LEGO-Eval), define
\begin{equation}
\label{eq:synergy_s_def}
 s_0 = s(M_0),\; s_R = s(M_R),\; s_C = s(M_C),\; s_{R+C} = s(M_{R+C}).
\end{equation}
The independent contribution of each module over the baseline is
\begin{equation}
\label{eq:synergy_delta_def}
 \Delta_R = s_R - s_0,\quad \Delta_C = s_C - s_0,\quad \Delta_{R+C} = s_{R+C} - s_0.
\end{equation}

\paragraph{Weak Synergy Gain (WSG).}
WSG asks whether the full system beats the better of the two single-module variants:
\begin{equation}
\label{eq:wsg}
 \mathrm{WSG}_s = s_{R+C} - \max\{s_R,\, s_C\}.
\end{equation}
$\mathrm{WSG}_s > 0$ rules out the trivial explanation that one pillar subsumes the other.

\paragraph{Additive Synergy Gain (ASG).}
ASG asks whether the joint improvement exceeds the sum of the two independent improvements:
\begin{equation}
\label{eq:asg}
 \mathrm{ASG}_s = \Delta_{R+C} - (\Delta_R + \Delta_C) = s_{R+C} - s_R - s_C + s_0.
\end{equation}
$\mathrm{ASG}_s > 0$ indicates a super-additive interaction.

\paragraph{Empirical reading.}
On LEGO-Eval, the full LEGO system is better than either single-module variant under both metrics (i.e., $\mathrm{WSG}_{\text{Acc}} > 0$ and $\mathrm{WSG}_{\text{F1}} > 0$), indicating clear synergy between retrieval and reasoning.
The stronger super-additivity condition holds for F1 but not for Acc: $\mathrm{ASG}_{\text{F1}} > 0$, while Acc is approximately additive (slightly sub-additive).

This asymmetry is mechanistically interpretable. Without retrieval context, structured expert reasoning can push the model toward overly decisive multi-label commitments, which can slightly hurt samples-F1; once ExpertGraphRAG supplies the controlling rule and its normative neighbourhood, the same structured reasoning becomes a lever for higher-precision multi-label verdicts, yielding a super-additive F1 gain. By contrast, on Acc both modules already yield sizable individual improvements, so the combined gain is close to additive rather than strongly super-additive.
